# Supplementary material for: Novel Class Discovery for Ultra-Fine-Grained Visual Categorization
Source: arXiv:2405.06283 source file (2024-05-10)
Supplement: Supplementary file 1 [file X_suppl.tex]

\clearpage
\setcounter{page}{1}
\maketitlesupplementary

\section{More on Algorithm Procedure}
In addition to the details elaborated in the main paper, we present the training procedure of our two-stage RAPL framework that includes three main designs for UFG-NCD, \ie, channel-wise region alignment (CRA), proxy-guided supervised learning (PSL) and proxy-guided contrastive learning (PCL).
The detailed training procedure of the pre-train phase and the discover phase is shown in~\cref{algorithm:pre-train,algorithm:discover} respectively. 
Note that, we first pre-train the whole network on labeled split with the objective in~\cref{eq:pre-train}, and then fine-tune the model on the combination of labeled and unlabeled splits with the objective in~\cref{eq:discover}.
In order to obtain more algorithmic details and reproduce the results reported in~\cref{tab:task-agnostic,tab:task-aware}, please refer to the source code included in the supplementary material. 

\begin{algorithm}
\DontPrintSemicolon
  \SetAlgoLined
  \KwIn {Feature Extractor $f$, Projection Head (with Global Average Pooling) $h$, Labeled split $\mathcal{D}^l$, Old proxies $\mathcal{P}^{old}$.}
  \KwOut {$f$, $h$, $\mathcal{P}^{old}$.}
  Randomly initialize $f$, $h$, $\mathcal{P}^{old}$;\\
  \For {$n = 1$ in $[1, max\_epoch\_pre-train]$}{
    \For {$i = 1$ in $[1,max\_iteration]$}{
    Sample labeled mini-batches $X^l$ from $D^l$;\\
    Extract feature maps $Q^l$;\\
    Group and assign region label for each feature matrix $z$ in $Z\in Q^l$;\\
    Calculate $\mathcal{L}^{CRA}$ by~\cref{eq:cra};\\
    Generate feature vector $V^l$ by $V^l=h(\text{flatten}(Q^l)$;\\
    Construct similarity matrix $S$ between $V^l$ and $\mathcal{P}^{old}$ by~\cref{eq:similarity_sample_to_proxy};\\
    Generate top-$k$ negative mask $M$ by~\cref{eq:mask_m};\\
    Perform mask scale softmax by~\cref{eq:sacle_mask_softmax} on the selected similarities by~\cref{eq:select_similarity};\\
    Calculate $\mathcal{L}^{PC}$ by~\cref{eq:pc};\\
    Construct similarity matrix $S^p$ within $\mathcal{P}^{old}$ by~\cref{eq:similarity_proxy_to_proxy};\\
    Calculate $\mathcal{L}^{REG}$ by~\cref{eq:reg};\\
    Calculate overall optimization objective by~\cref{eq:pre-train};\\
    Update $f$, $h$ and $\mathcal{P}^{old}$ by SGD~\cite{sgd};\\
    }
  }
  \caption{Pre-train Phase of our RAPL}
  %\caption{Algorithm Pipeline of the pre-train phase in our RAPL}
  \label{algorithm:pre-train}
\end{algorithm}

\begin{algorithm}
\DontPrintSemicolon
  \SetAlgoLined
  \KwIn {Feature Extractor $f$, Projection Head (with Global Average Pooling) $h$, Labeled and Unlabeled splits $\mathcal{D}^l,\mathcal{D}^u$, Old and New proxies $\mathcal{P}^{old},\mathcal{P}^{new}$.}
  \KwOut {$f$, $h$, $\mathcal{P}^{old}$ and $\mathcal{P}^{new}$.}
  Initialize $\mathcal{P}^{new}$ by $k$-means~\cite{kmeans}.\\
  \For {$n = 1$ in $[1, max\_epoch\_discover]$}{
    \For {$i = 1$ in $[1,max\_iteration]$}{
    Sample labeled and unlabeled mini-batches $[X^l,X^u]$ from $D^l\cup D^u$;\\
    Extract feature maps $Q=[Q^l,Q^u]$;\\
    Group and assign region label for each feature matrix $z$ in $Z\in Q$;\\
    Calculate $\mathcal{L}^{CRA}$ by~\cref{eq:cra};\\
    Generate feature vector $V=[V^l,V^u]$ by $V=h(\text{flatten}(Q)$;\\
    Construct similarity matrix $S$ between $V^l$ and $\mathcal{P}^{old}$ by~\cref{eq:similarity_sample_to_proxy};\\
    Generate top-$k$ negative mask $M$ by~\cref{eq:mask_m};\\
    Perform mask scale softmax by~\cref{eq:sacle_mask_softmax} on the selected similarities by~\cref{eq:select_similarity};\\
    Calculate $\mathcal{L}^{PC}$ on by~\cref{eq:pc};\\
    Calculate $\mathcal{L}^{PCL}$ by~\cref{eq:pcl};\\
    Calculate overall optimization objective by~\cref{eq:discover};\\
    Update $f$, $h$ and $\mathcal{P}^{new}$ by SGD~\cite{sgd};\\
    }
  }
  \caption{Discover Phase of our RAPL}
  %\caption{Algorithm Pipeline of the discover phase in our RAPL}
  \label{algorithm:discover}
\end{algorithm}

\begin{figure*}[t]
  \centering
  %\hfill
  \begin{subfigure}{0.33\linewidth}
    %\centering
    \includegraphics[width=1\linewidth]{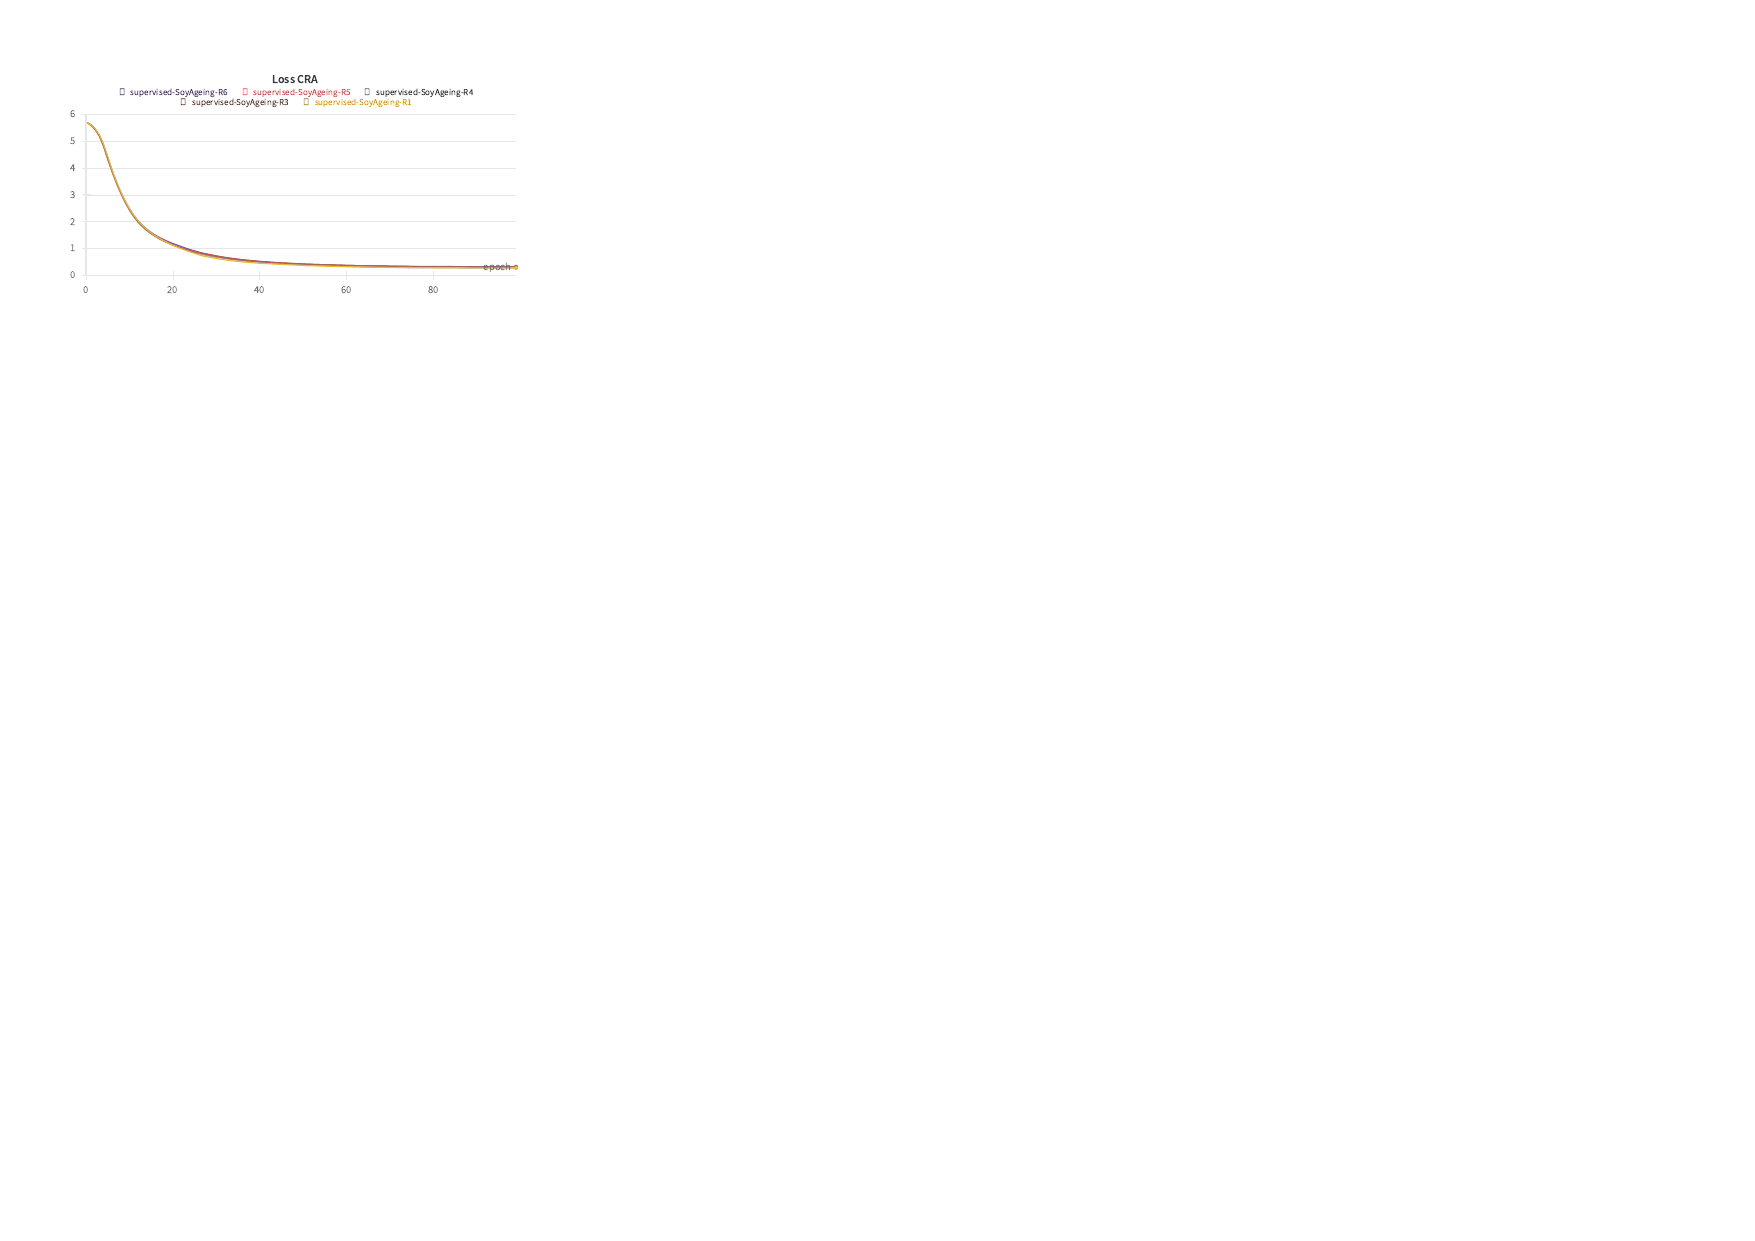}
    \caption{$\mathcal{L}^{CRA}$}
    \label{fig:supcra}
  \end{subfigure}
  \begin{subfigure}{0.33\linewidth}
    %\centering
    \includegraphics[width=1\linewidth]{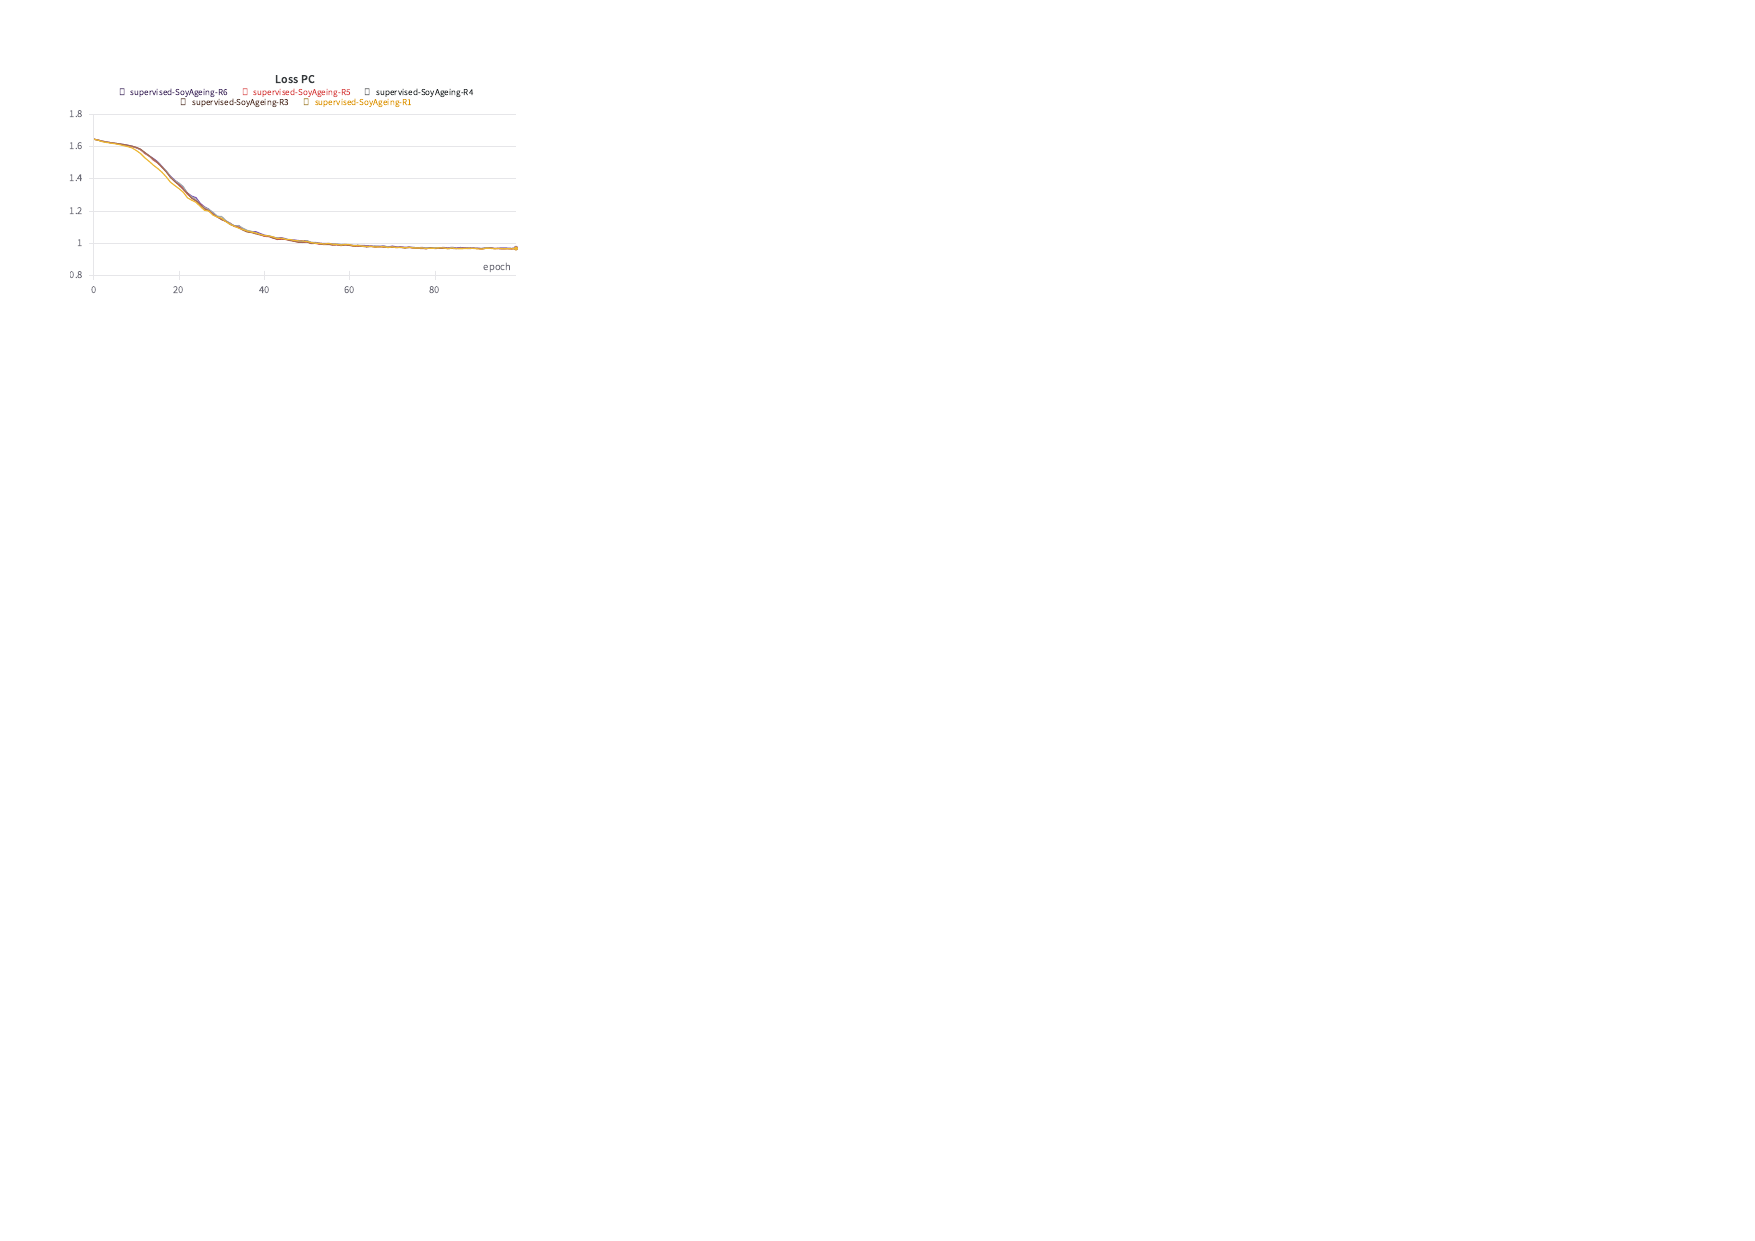}
    \caption{$\mathcal{L}^{PC}$}
    \label{fig:suppc}
  \end{subfigure}
  \begin{subfigure}{0.33\linewidth}
    %\centering
    \includegraphics[width=1\linewidth]{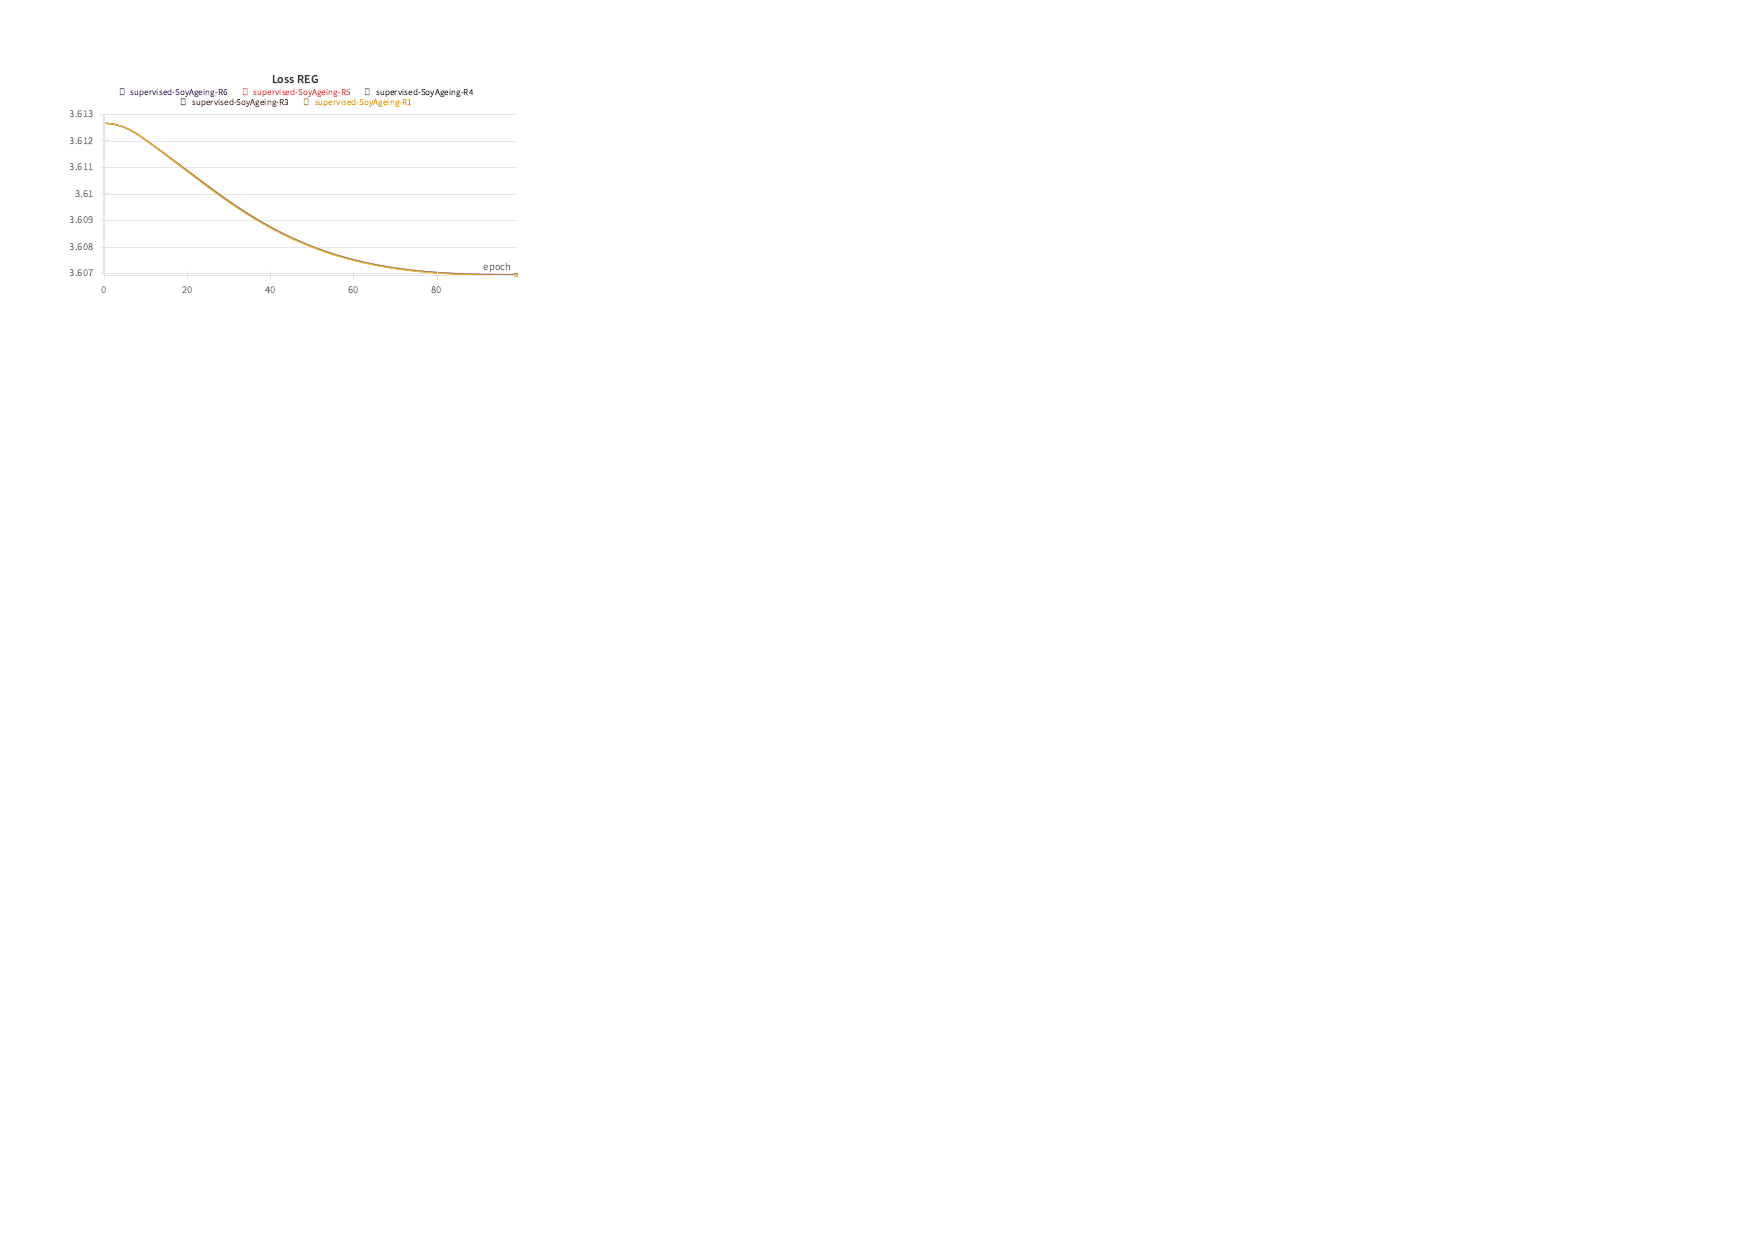}
    \caption{$\mathcal{L}^{REG}$}
    \label{fig:supreg}
  \end{subfigure}
  \caption{We show the loss curves in the pre-train phase on five UFG-NCD datasets, where the x-axis indicates the training epochs and the y-axis is the loss cost for each loss as~\cref{eq:cra,eq:pc,eq:reg}}
  \label{fig:preloss}
\end{figure*}

\begin{figure*}[t]
  \centering
  %\hfill
  \begin{subfigure}{0.33\linewidth}
    %\centering
    \includegraphics[width=1\linewidth]{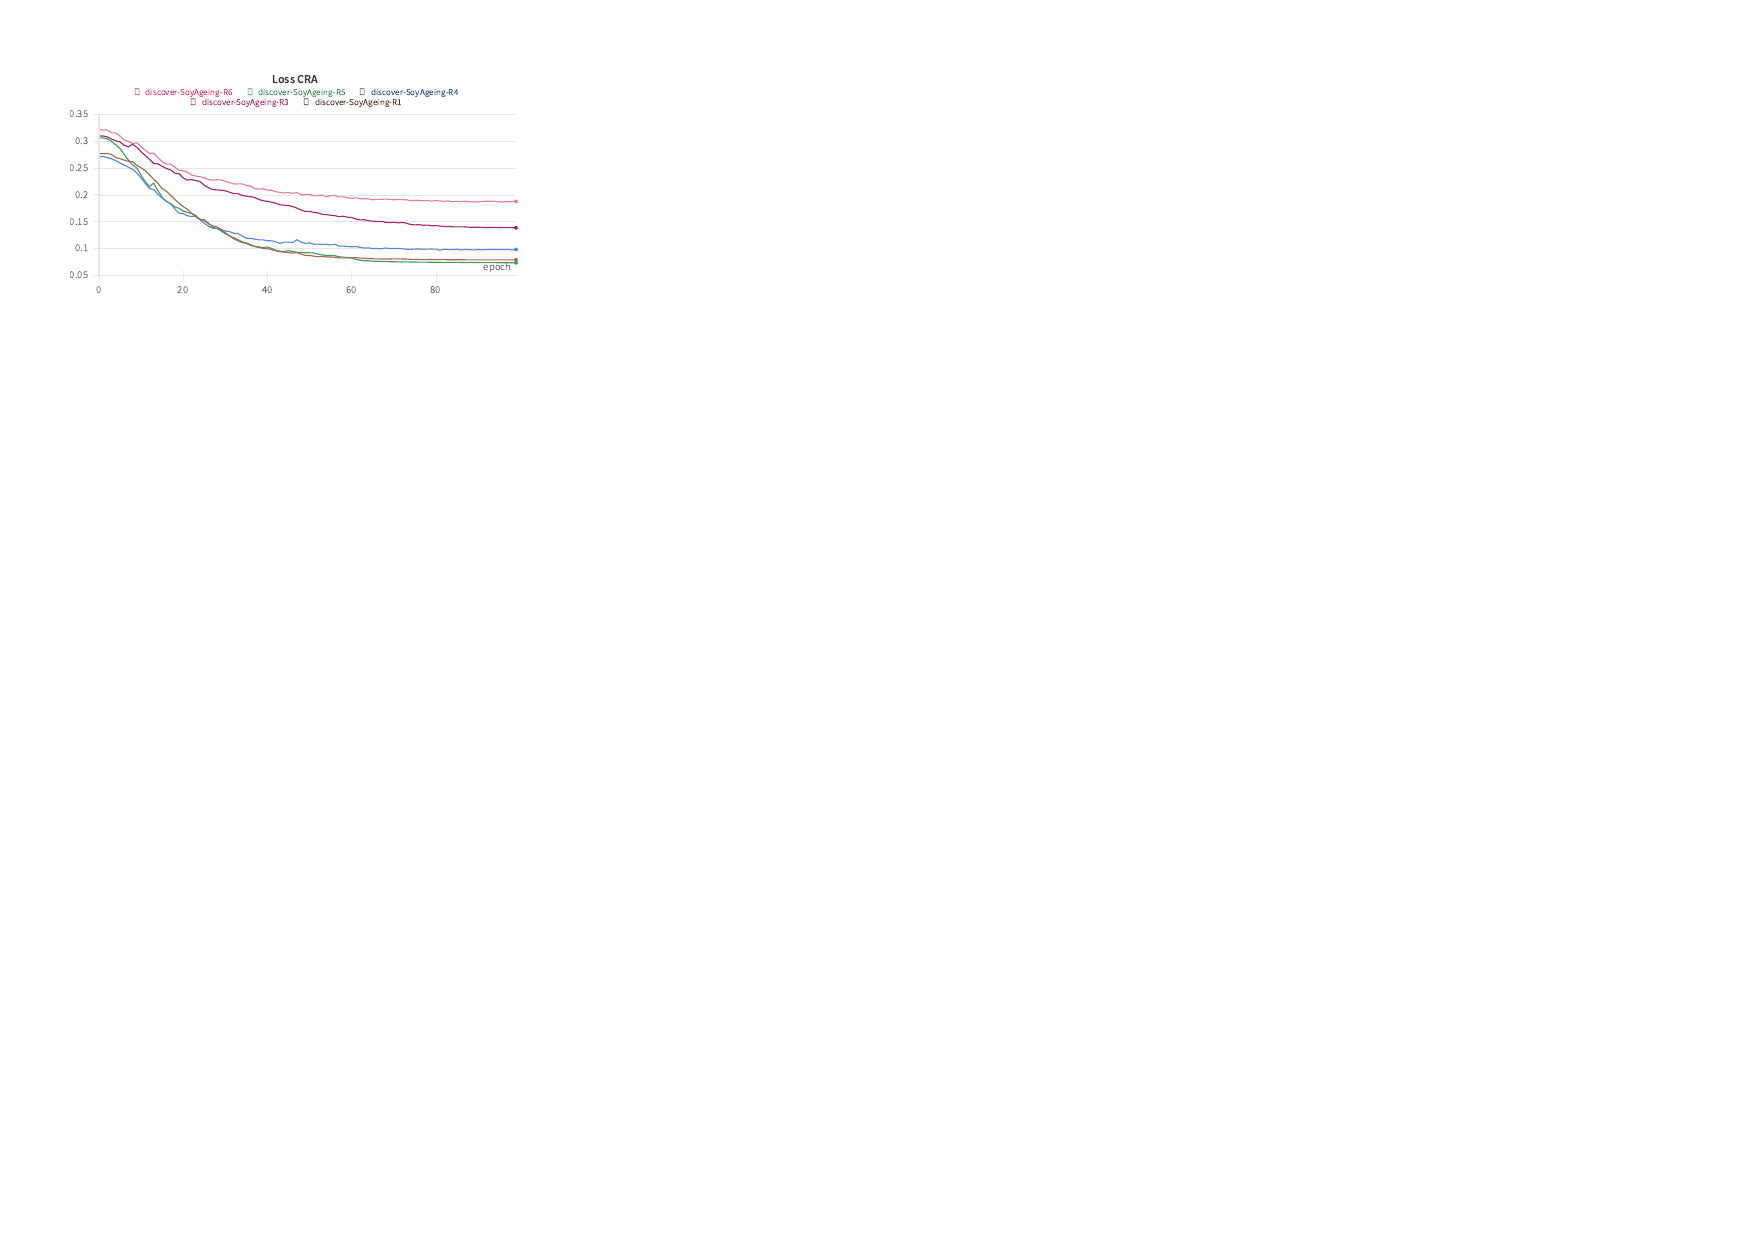}
    \caption{$\mathcal{L}^{CRA}$}
    \label{fig:discra}
  \end{subfigure}
  \begin{subfigure}{0.33\linewidth}
    %\centering
    \includegraphics[width=1\linewidth]{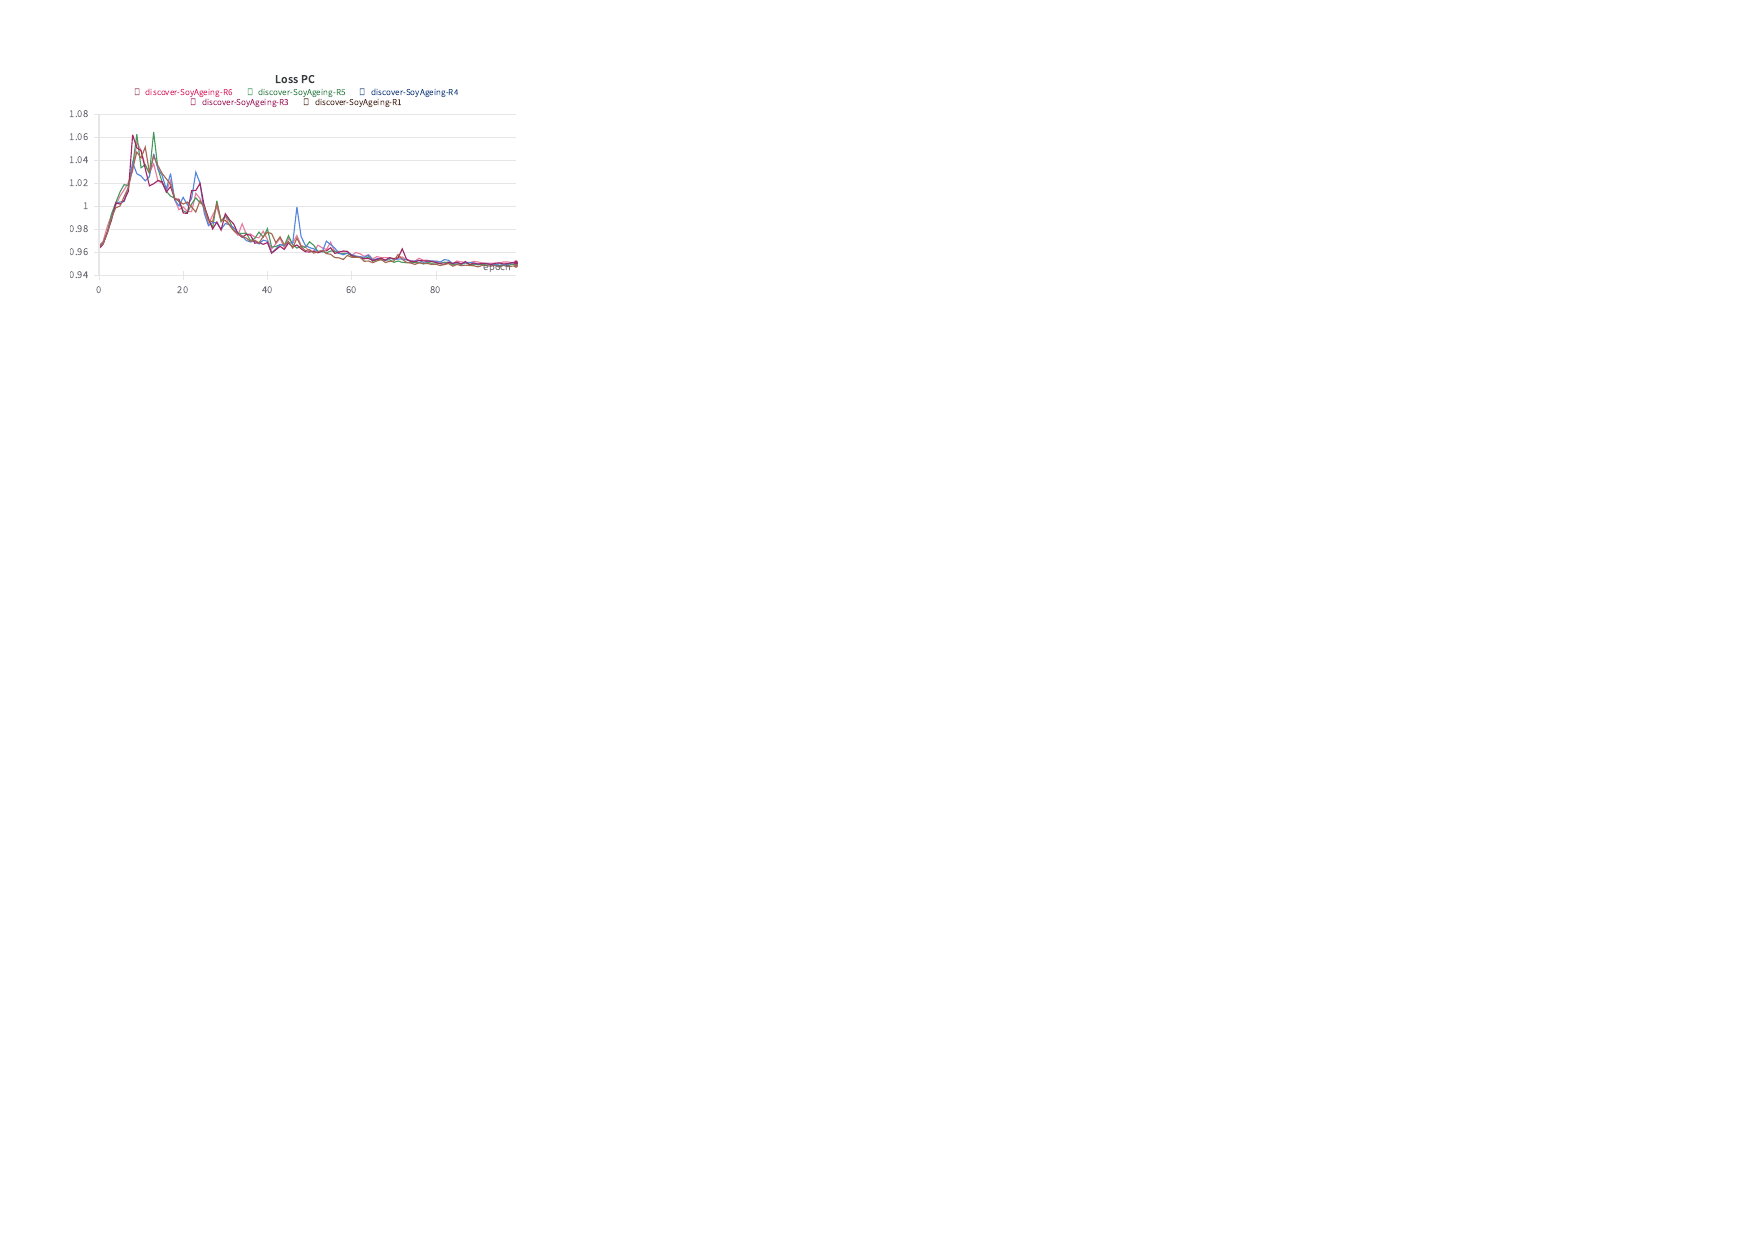}
    \caption{$\mathcal{L}^{PC}$}
    \label{fig:dispc}
  \end{subfigure}
  \begin{subfigure}{0.33\linewidth}
    %\centering
    \includegraphics[width=1\linewidth]{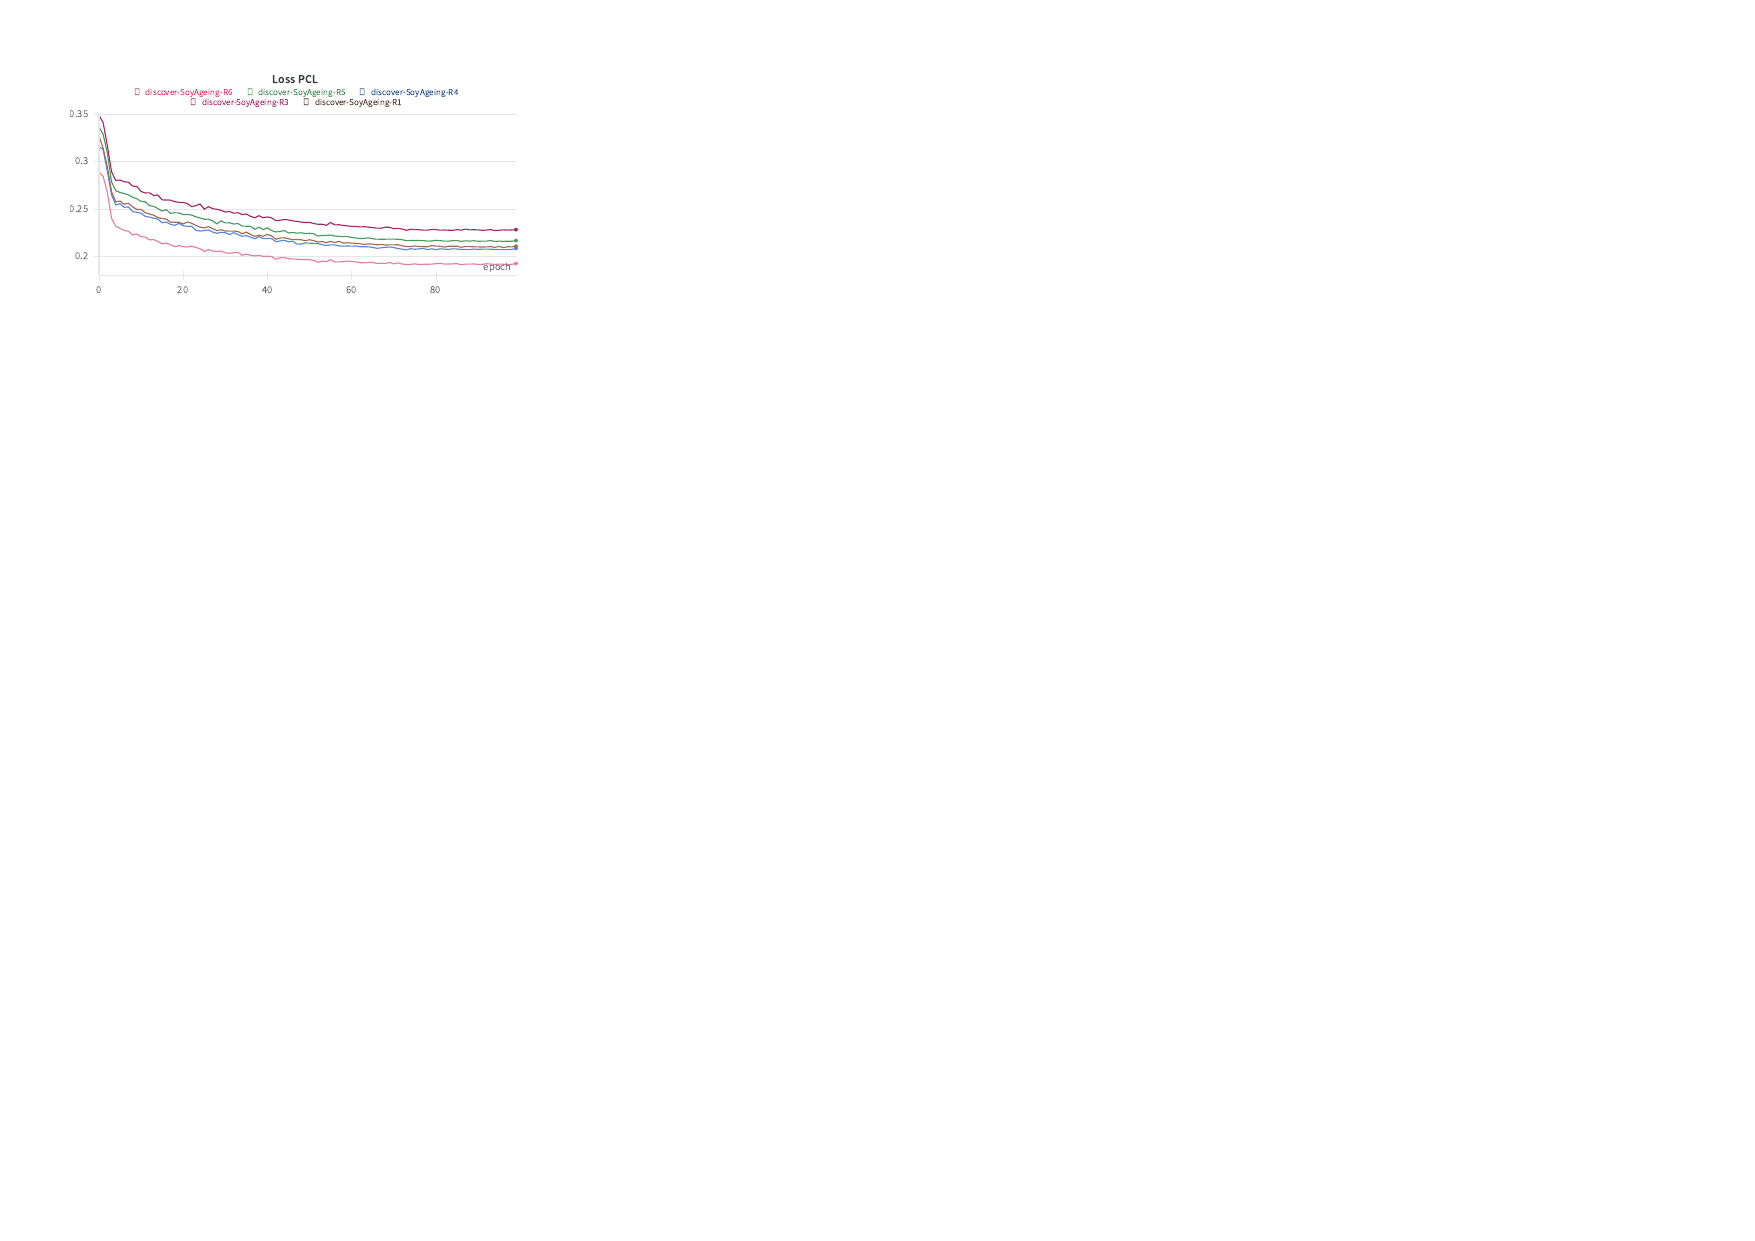}
    \caption{$\mathcal{L}^{PCL}$}
    \label{fig:dispcl}
  \end{subfigure}
  
  \caption{We show the loss curves in the discover phase on five UFG-NCD datasets, where x-axis indicates the training epochs and y-axis is the loss cost for each loss as~\cref{eq:cra,eq:pc,eq:pcl}}
  \label{fig:disloss}
\end{figure*} 

\begin{table*}[t]
  \centering
  \begin{adjustbox}{width=1\linewidth}
    \begin{tabular}{c|ccccc|cccccccccccccccccc}
      \toprule
      & \multicolumn{5}{c}{Component} & \multicolumn{3}{|c}{SoyAgeing-R1} &  \multicolumn{3}{c}{SoyAgeing-R3} &  \multicolumn{3}{c}{SoyAgeing-R4} & \multicolumn{3}{c}{SoyAgeing-R5} & \multicolumn{3}{c}{SoyAgeing-R6} &  \multicolumn{3}{c}{Average}\\
      \cmidrule(lr){2-6}\cmidrule(lr){7-9}\cmidrule(lr){10-12}\cmidrule(lr){13-15}\cmidrule(lr){16-18}\cmidrule(lr){19-21}\cmidrule(lr){22-24}
      & $\mathcal{L}^{PC}$ & $\mathcal{L}^{REG}$ & $\mathcal{L}^{CRA}$ & $\mathcal{L}^{PCL}$ & $\mathcal{L}^{VCL}$ & All & Old & New & All & Old & New & All & Old & New & All & Old & New & All & Old & New & All & Old & New\\
      \midrule
      (1) & \checkmark & \checkmark & \checkmark & & \checkmark & 56.36 & 74.14 & 38.59 & 54.34 & 74.75 & 33.94 & 56.46 & 74.14 & 38.79 & 55.86 & 72.53 & 39.19 & 48.28 & 62.63 & 33.94 & 54.26 & 71.64 & 36.89\\
      (2) & \checkmark & \checkmark & & \checkmark & & 56.97 & 75.56 & 38.38 & \textbf{58.99} & \textbf{78.79} & 39.19 & 56.46 & 72.73 & 40.20 & 55.96 & 72.32 & 39.60 & 47.98 & 60.81 & 35.15 & 55.27 & 72.04 & 38.50\\
      (3) & \checkmark & & \checkmark & \checkmark & & 58.48 & 76.97 & \textbf{40.00} & 57.37 & 76.16 & 38.59 & \textbf{58.69} & \textbf{74.34} & \textbf{43.03} & 57.78 & \textbf{74.75} & 40.81 & \textbf{52.12} & \textbf{66.87} & \textbf{37.37} & 56.89 & \textbf{73.82} & 39.96\\
      (4) & \checkmark & \checkmark & \checkmark & \checkmark & & \textbf{58.99} & \textbf{79.19} & 38.79 & \textbf{58.99} & 78.59 & \textbf{39.39} & 57.07 & 71.92 & 42.22 & \textbf{61.01} & \textbf{74.75} & \textbf{47.27} & 50.20 & 64.65 & 35.76 & \textbf{57.25} & \textbf{73.82} & \textbf{40.69}\\
      \bottomrule
    \end{tabular}
  \end{adjustbox}
\caption{Ablation study on all UFG-NCD datasets. Each component of our method is removed in isolation, where $\mathcal{L}^{VCL}$ indicates vanilla contrastive learning without the guidance of proxies.}
\label{ablation_more}
\end{table*}

\section{More on Experimental Deatils}
\subsection{Implementation Details on RAPL}
To obtain more discriminative representation, we use a stronger feature extractor and higher resolution images than the general implementation of NCD. 
Specifically, we train all methods using a ResNet-50~\cite{resnet} backbone with ImageNet~\cite{imagenet} pre-trained weights on 448 $\times$ 448 resolution images. 
Furthermore, following~\cite{ultra-cle-vit23}, in the training process, the input images are cropped with a random scale within $\{0.67,1.0\}$ and then resized to 448 $\times$ 448.
After that, we perform random data augmentation to generate two views of each image, which includes horizontal flip, vertical flip, ``ColorJitter'', ``Grayscale'' and ``GaussianBlur''. 
While in the inference process, images are simply resized to 512 $\times$ 512 and center-cropped into 448 $\times$ 448. 
Due to the backbone and image resolution, we used in UFG-NCD, the feature map $ Z\in \mathbb{R}^{2048\times14\times14}$, and feature vector $v \in \mathbb{R}^{2048}$.
Thus, we divide the feature maps into $H * W=196$ groups to encode the features of all regions. 
To make the feature dimensions consistent, \ie, $D=2048$, the first 108 groups of feature maps each have 10 feature maps and the remaining groups each have 11 feature maps, denoted as:
\begin{equation}
   \hat{Z}^i \in 
   \begin{cases}
       \mathbb{R}^{10\times14\times14}, &\text{if~}i < 108 \\
       \mathbb{R}^{11\times14\times14}, &\text{if~}i \geq 108 ~\text{and}~ i < 196.
   \end{cases}
   \label{eq:groups}
\end{equation}
%$\hat{Z}^i \in \mathcal{10\times14\times14}, i\in[0,..,107]$.

Following~\cite{gcd-gcd}, we use a three-layer MLP projection head to facilitate representation learning of PSL and PCL in the embedding space, in which the input and output dimensions are both 2048, and the hidden dimension is set to 10240 for richer representation embedding. 

Moreover, we illustrate the training loss curves on five UFG-NCD datasets in the pre-train and the discover phase of our RAPL in~\cref{fig:preloss,fig:disloss} respectively.
Specifically, as shown in~\cref{fig:preloss}, the decline of each training loss in~\cref{eq:pre-train} is quite rapid in the early stage of the pre-train phase due to full supervision.
Then, the decrease of these loss gradually slow down as training progress, and shows a stable convergence trend eventually. 
On the other hand, $\mathcal{L}^{CRA}$ and $\mathcal{L}^{PCL}$ show similar trendency in the discover phase.
However, the proxy-guided classification loss $\mathcal{L}^{PC}$ shows a trend of first increasing and then decreasing due to the representation learning of the new incoming unlabeled data.

% \begin{figure*}[t]
%   \centering
%   %\hfill
%   \begin{subfigure}{1\linewidth}
%     %\centering
%     \includegraphics[width=1\linewidth]{pictures suppl/CRA_SoyAgeing-R1.pdf}
%    \caption{Visualization on 8 cultivars from SoyAgeing-R1.}
%    \label{fig:cra-soyageing-r1}
%   \end{subfigure}
%   \begin{subfigure}{1\linewidth}
%    \includegraphics[width=1\linewidth]{pictures suppl/CRA_SoyAgeing-R3.pdf}
%    \caption{Visualization on 8 cultivars from SoyAgeing-R3.}
%    \label{fig:cra-soyageing-r3}
%   \end{subfigure}
%   \caption{Visualization of top-15 groups of feature maps.}
%   \label{fig:cra-visual-13}
% \end{figure*}

\begin{figure*}[t]
  \centering
  %\hfill
  \begin{subfigure}{1\linewidth}
    %\centering
    \includegraphics[width=1\linewidth]{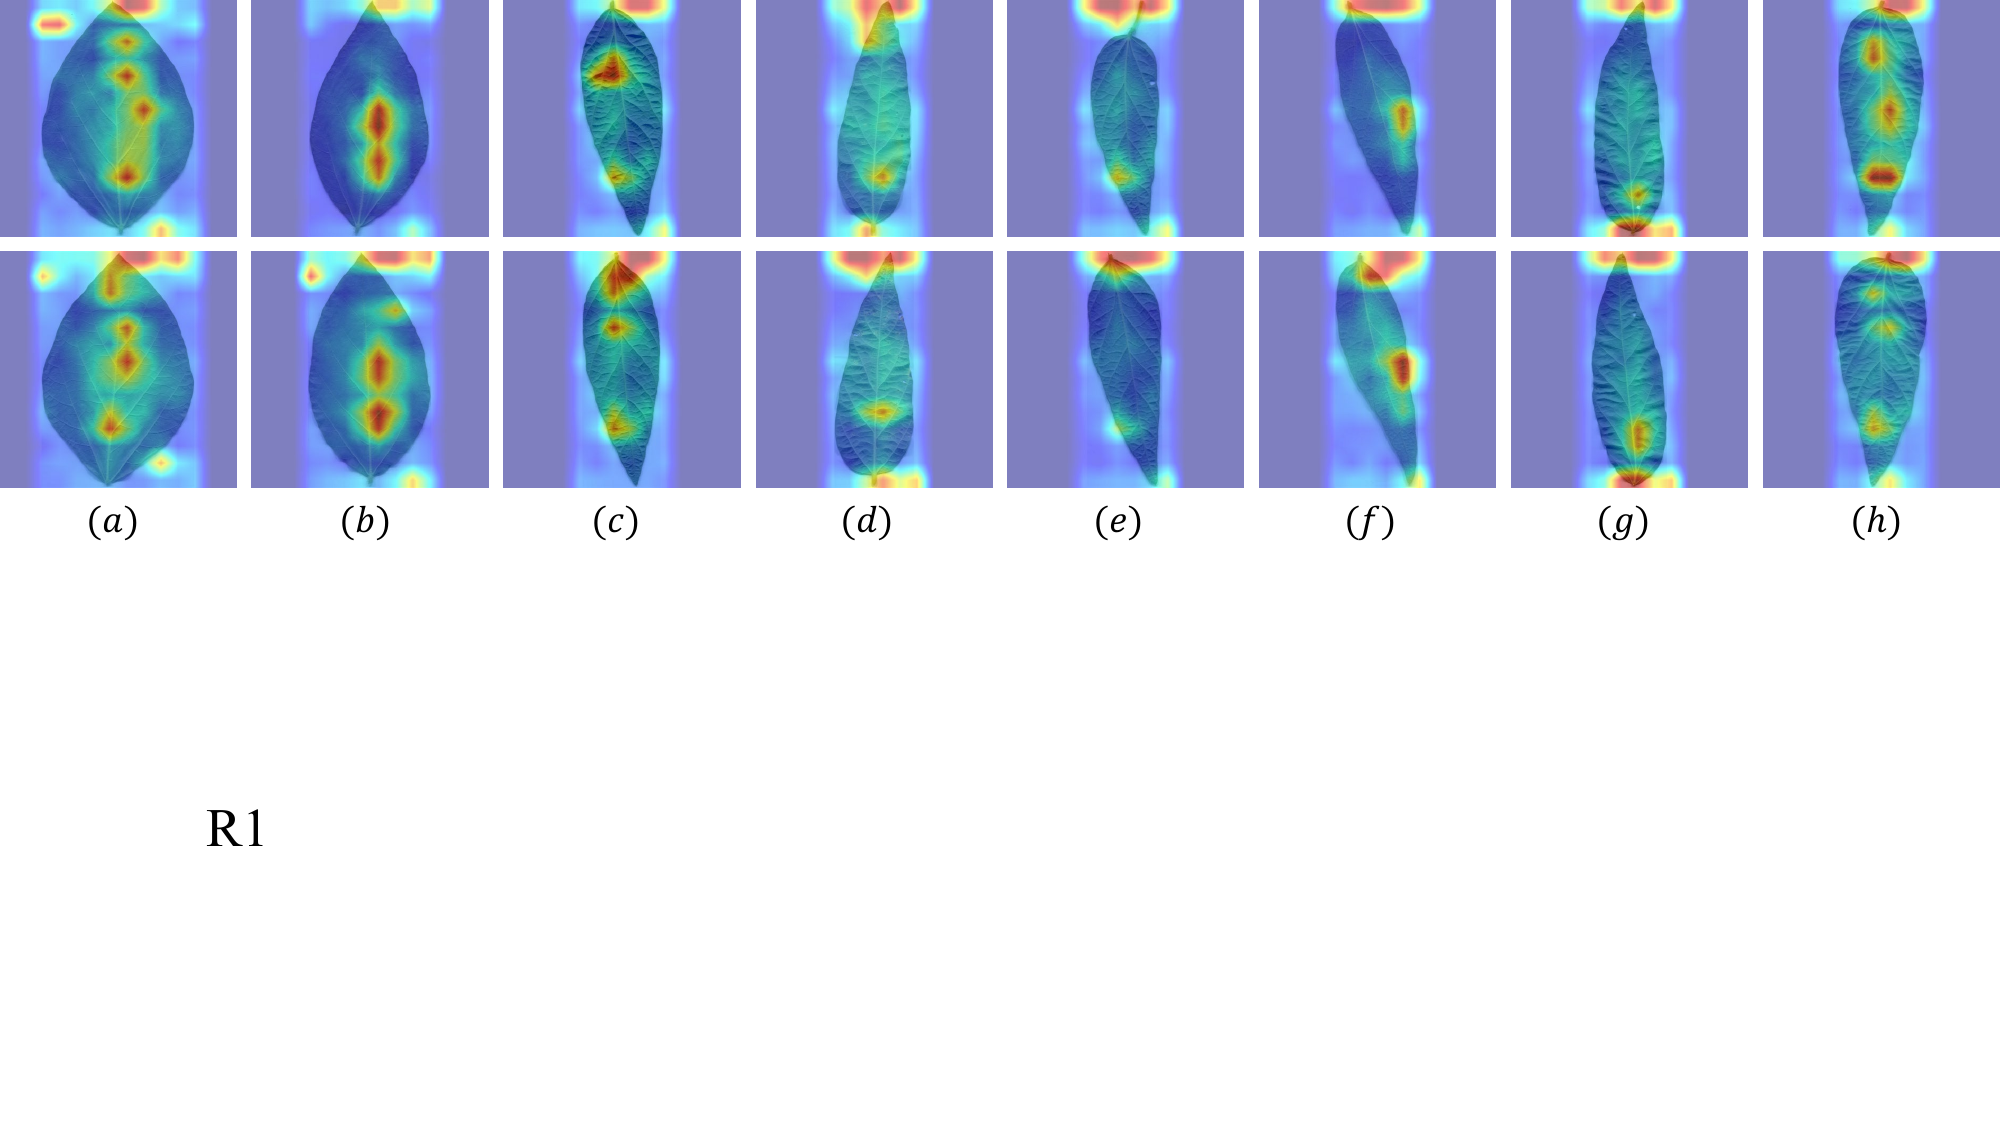}
   \caption{Visualization on 8 cultivars from SoyAgeing-R1.}
   \label{fig:cra-soyageing-r1}
  \end{subfigure}
  \begin{subfigure}{1\linewidth}
   \includegraphics[width=1\linewidth]{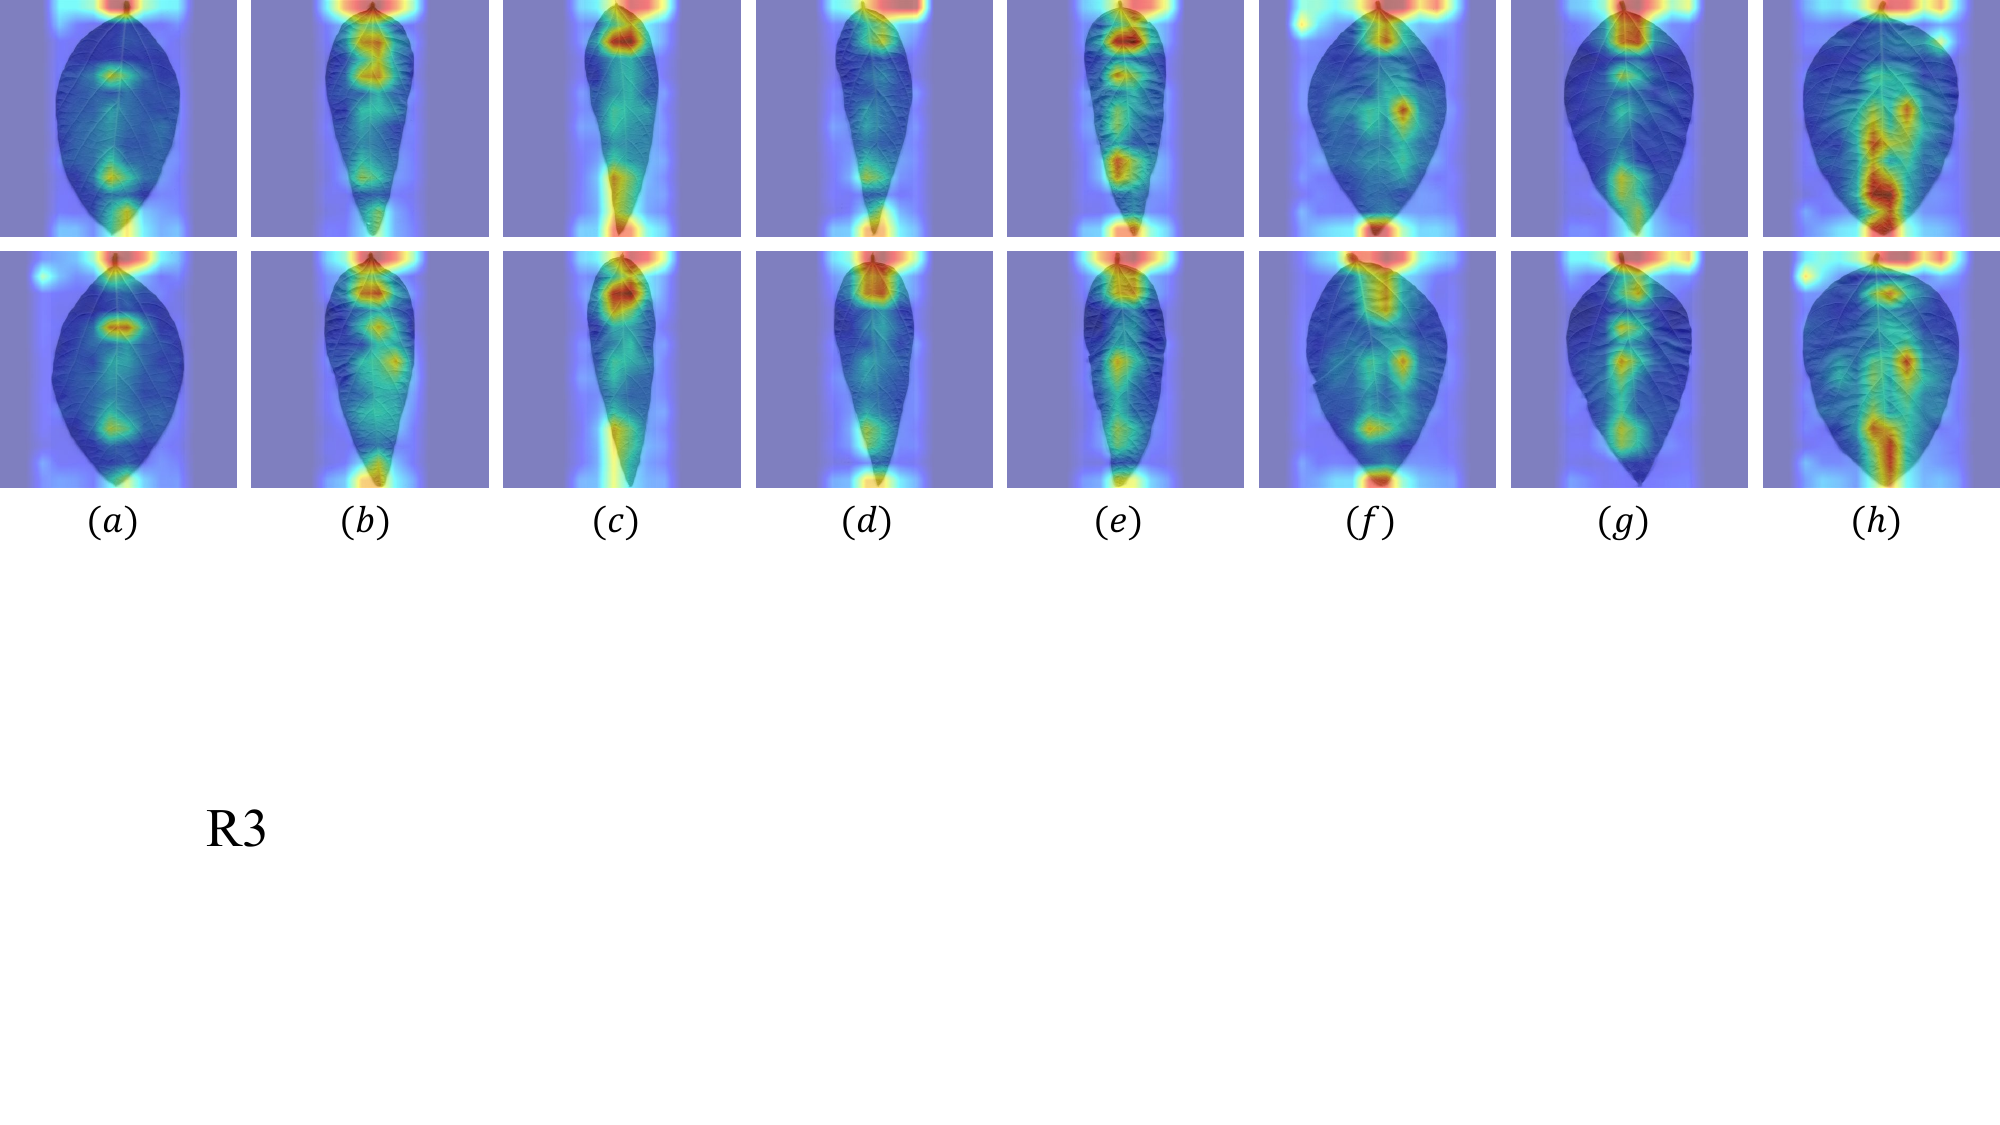}
   \caption{Visualization on 8 cultivars from SoyAgeing-R3.}
   \label{fig:cra-soyageing-r3}
  \end{subfigure}
  \caption{Visualization of top-15 groups of feature maps.}
  \label{fig:cra-visual-13}
\end{figure*}

\subsection{Implementation Details on Baselines}
We adopt five representative methods from novel class discovery (NCD) for our ultra-fine-grained novel class discovery (UFG-NCD) task. RankStat IL~\cite{ncd-rankstat} is widely used as a competitive baseline for NCD, while recent methods include state-of-the-art approaches are implemented based on UNO~\cite{ncd-uno}, \eg, ComEx~\cite{ncd-comex}, IIC~\cite{ncd-iic} and rKD~\cite{ncd-rkd}. 

In our study, we apply these NCD methods to the UFG-NCD task, leveraging their open-source code. 
We set the batch size into 32 for these baselines, and we train UNO, ComEX and IIC for 200 epochs in both training phases, and train RankStat IL and rKD for 100 in the pre-train phase, and 200/500 epochs in the discover phase respectively.
We fine-tuned the learning rates during each training phase to establish an optimized performance. 
Specifically, we set learning rates into \{0.1, 0.01, 0.001\} in the pre-train phase and the discover phase respectively, and report the best performance on these combinations of learning rates.
We report the optimal results of RankStat IL, UNO, ComEX and IIC when $lr_{pre-train}=0.01 $ and $lr_{discover}=0.1$. 
We report the results of rKD when $lr_{pre-train}=0.01 $ and $lr_{discover}=0.001$. 

\subsection{Details on Datasets.}
We choose five UFG-NCD datasets from~\cite{ultra-dataset21} in our experiments, namely SoyAgeing-\{R1, R3, R4, R5, R6\}.
For UFG-NCD, each class encompasses 5 images for both training and testing. Regarding GCD, there are 8 training images and 2 testing images per class, where unlabeled training data consists of 50\% of the images from $C^l$, in addition to all images from $C^u$, \ie, 1188 unlabeled training images contain 396 images from $C^l$ and 796 images from $C^u$.
We present the detailed statistics of the dataset in~\cref{tab:dataset}.

\section{More Results and Analysis}
\subsection{More on Ablation Results}
In addition to results on SoyAgeing-R1 (See in~\cref{ablation}), we present more ablation results on all UFG-NCD datasets by individually removing each component of RAPL in~\cref{ablation_more}.
Moreover, we report the average accuracy in terms of ``All'', ``Old'' and ``New'' in~\cref{ablation_more}, and the results demonstrate the effectiveness of each component of our RAPL.

\begin{table}[t]
\centering
\begin{adjustbox}{width=1\linewidth}
\begin{tabular}{ccccccc}
\toprule
\multirow{2}{*}{Task} & \multirow{2}{*}{$C^u$} & \multirow{2}{*}{$C^l$}& \multicolumn{2}{c}{Train} & \multicolumn{2}{c}{Test}\\
\cmidrule(lr){4-5}\cmidrule(lr){6-7}
 & & & $N^u$ & $N^l$ & $N^u$ & $N^l$ \\
\midrule
UFG-NCD & 99 & 99 & 495 & 495 & 495 & 495\\
GCD & 99 & 99 & 1188 & 396 & 196 & 196\\ 
\bottomrule
\end{tabular}
\end{adjustbox}
\caption{Statistics of the dataset splits of SoyAgeing-\{R1, R3, R4, R5, R6\} for UFG-NCD and GCD.}
\label{tab:dataset}
\end{table}

\begin{figure*}[t]
  \centering
  %\hfill
  \begin{subfigure}{1\linewidth}
    %\centering
    \includegraphics[width=1\linewidth]{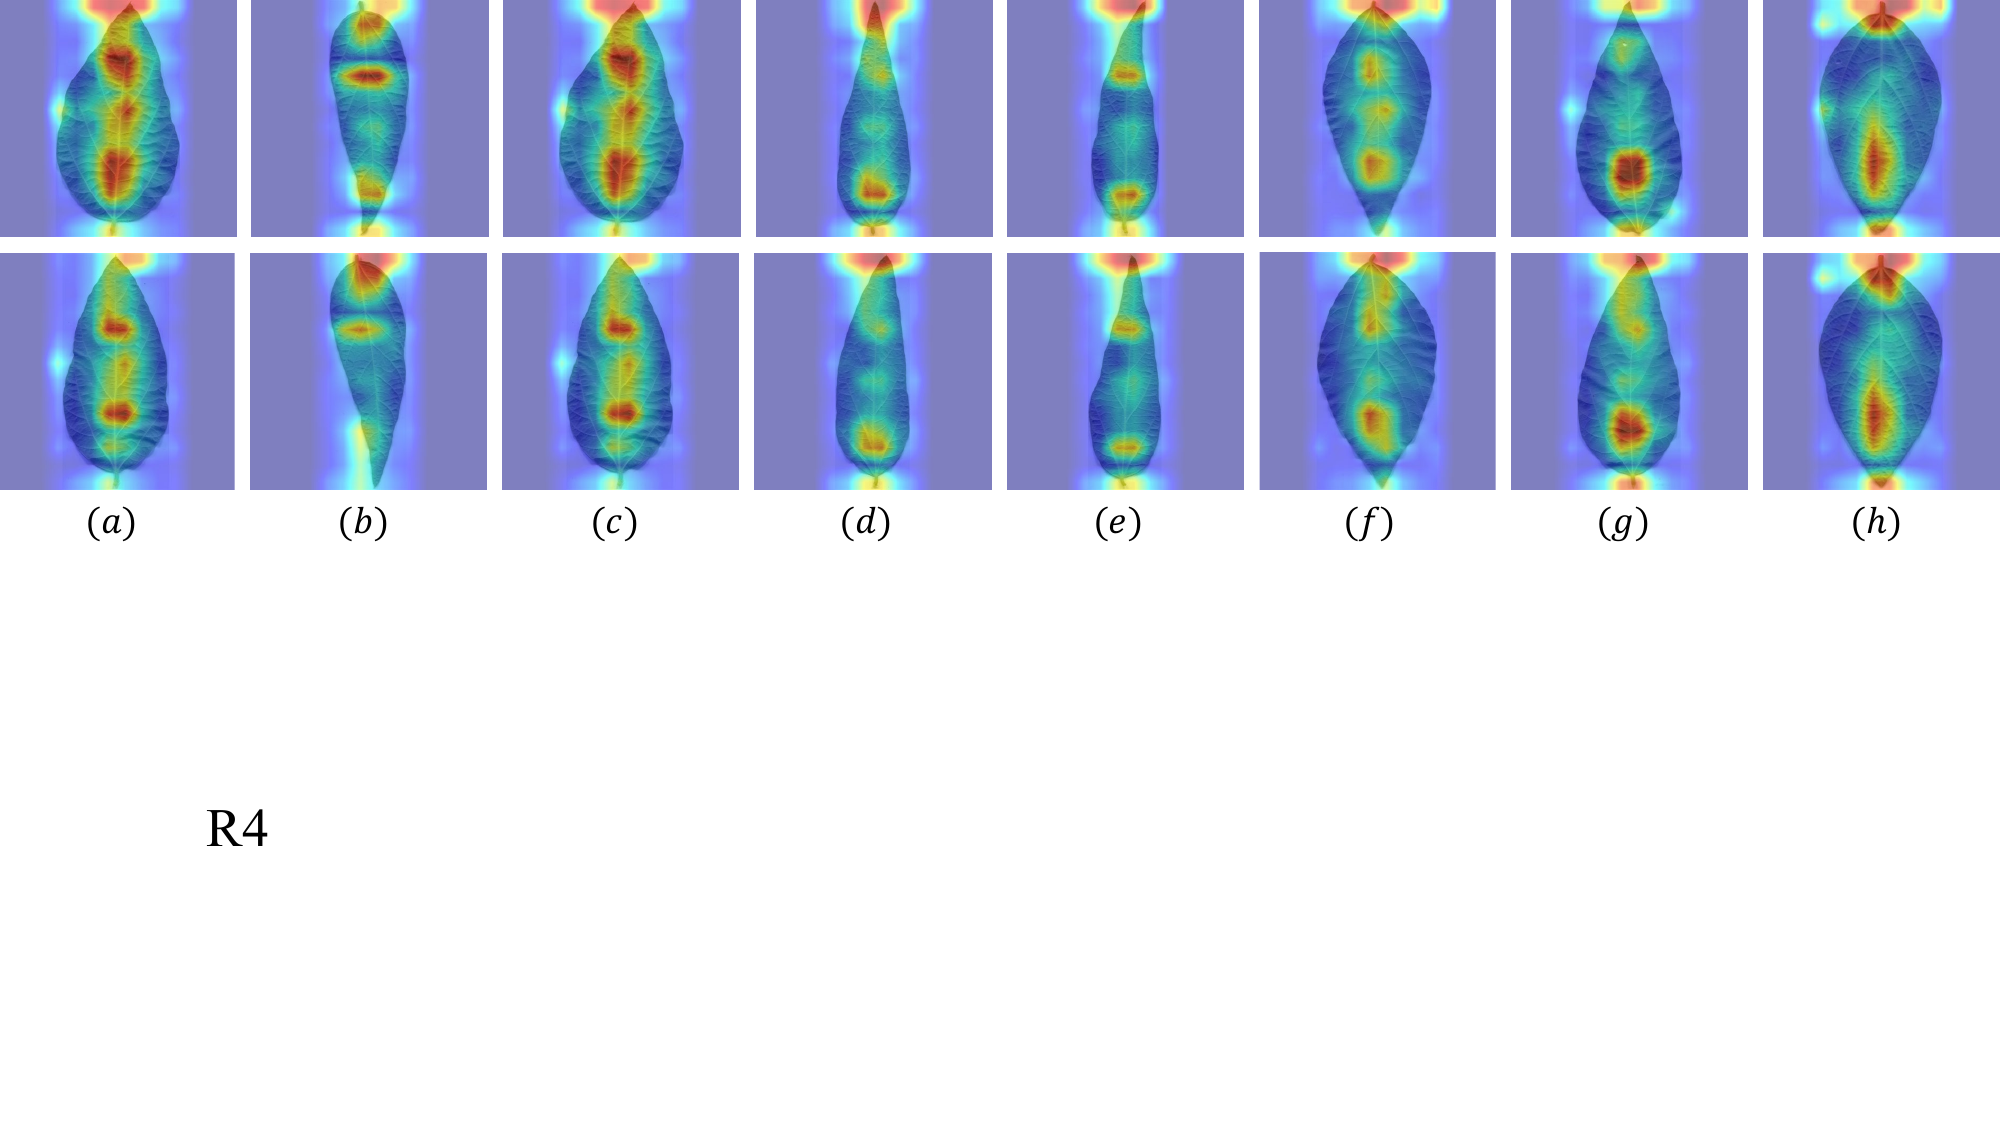}
   \caption{Visualization on 8 cultivars from SoyAgeing-R4.}
   \label{fig:cra-soyageing-r4}
  \end{subfigure}
  \begin{subfigure}{1\linewidth}
   \includegraphics[width=1\linewidth]{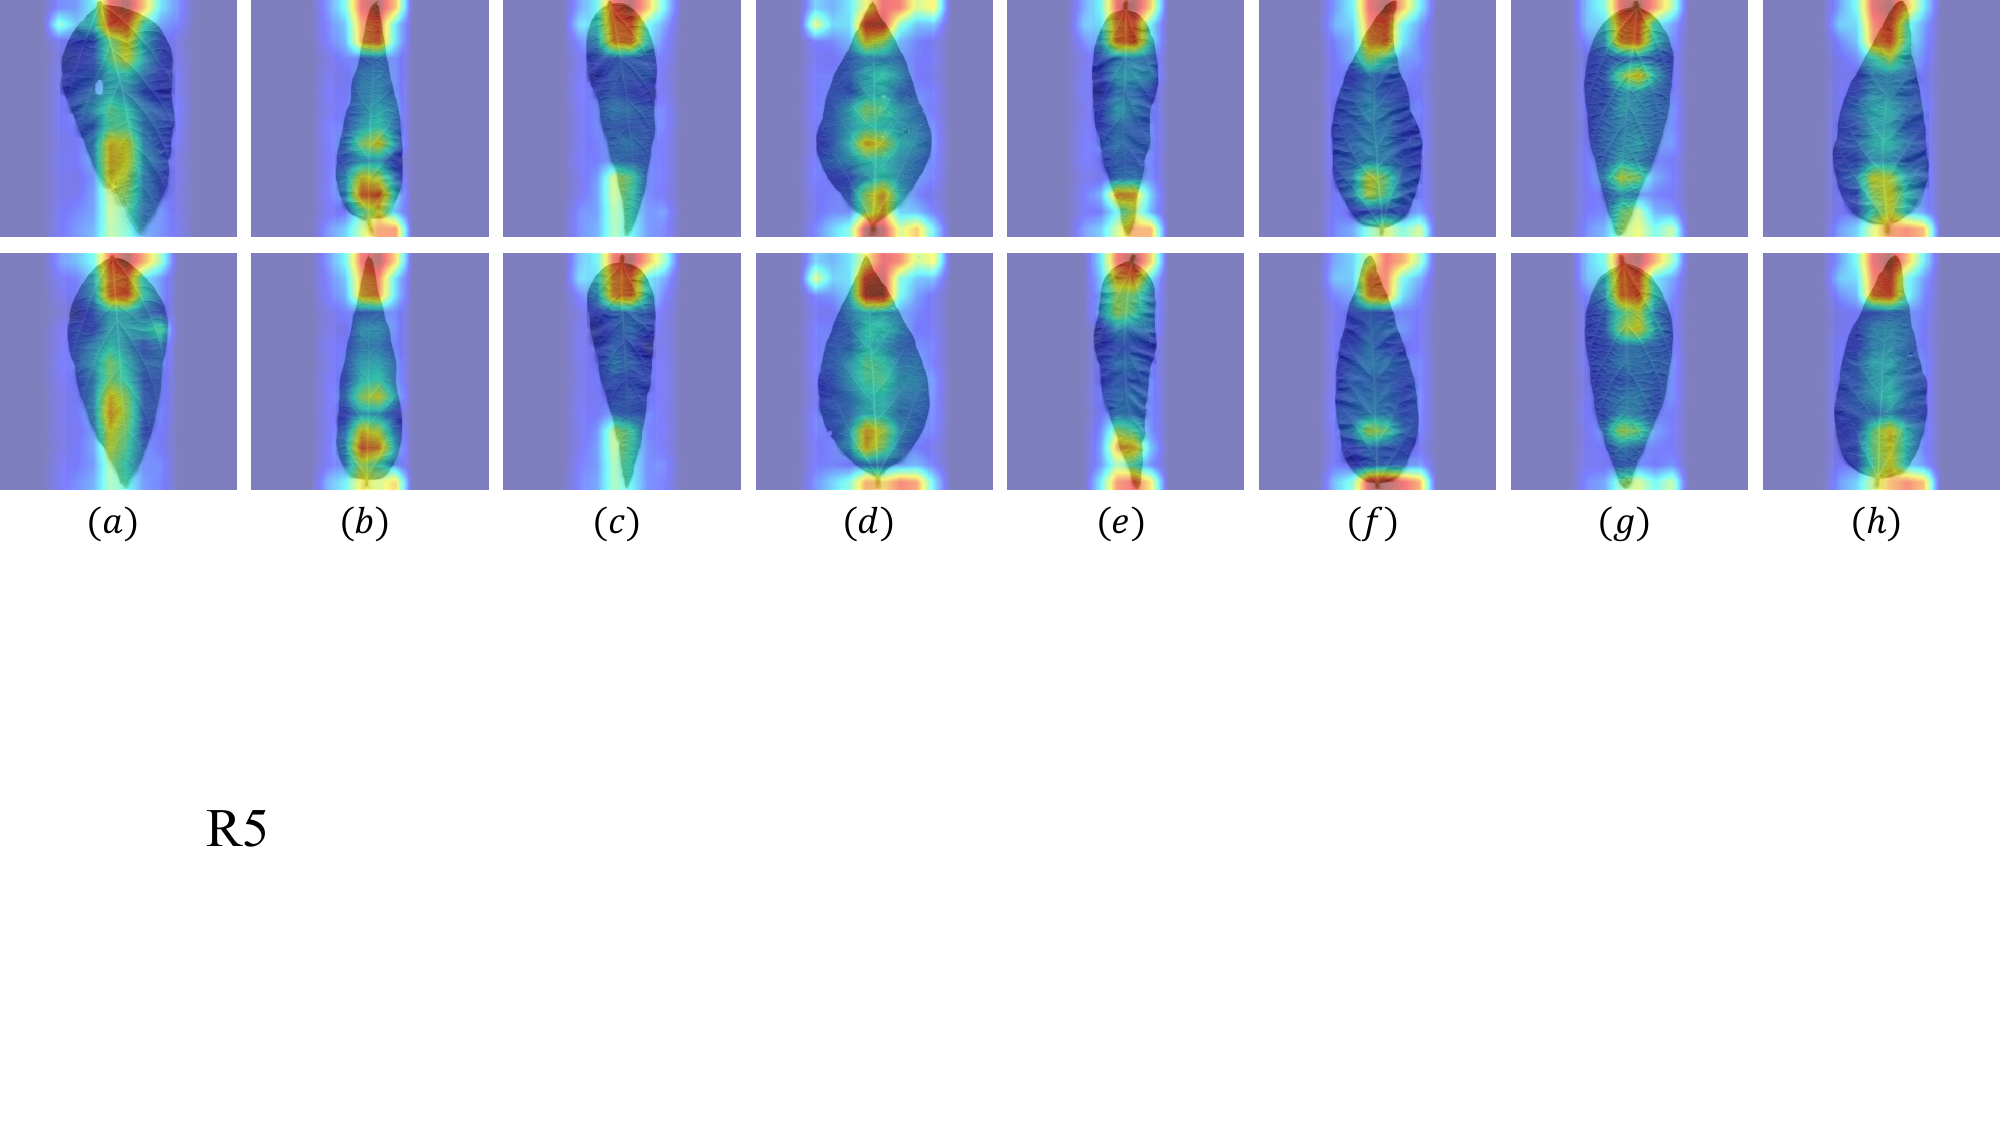}
   \caption{Visualization on 8 cultivars from SoyAgeing-R5.}
   \label{fig:cra-soyageing-r5}
  \end{subfigure}
  \begin{subfigure}{1\linewidth}
   \includegraphics[width=1\linewidth]{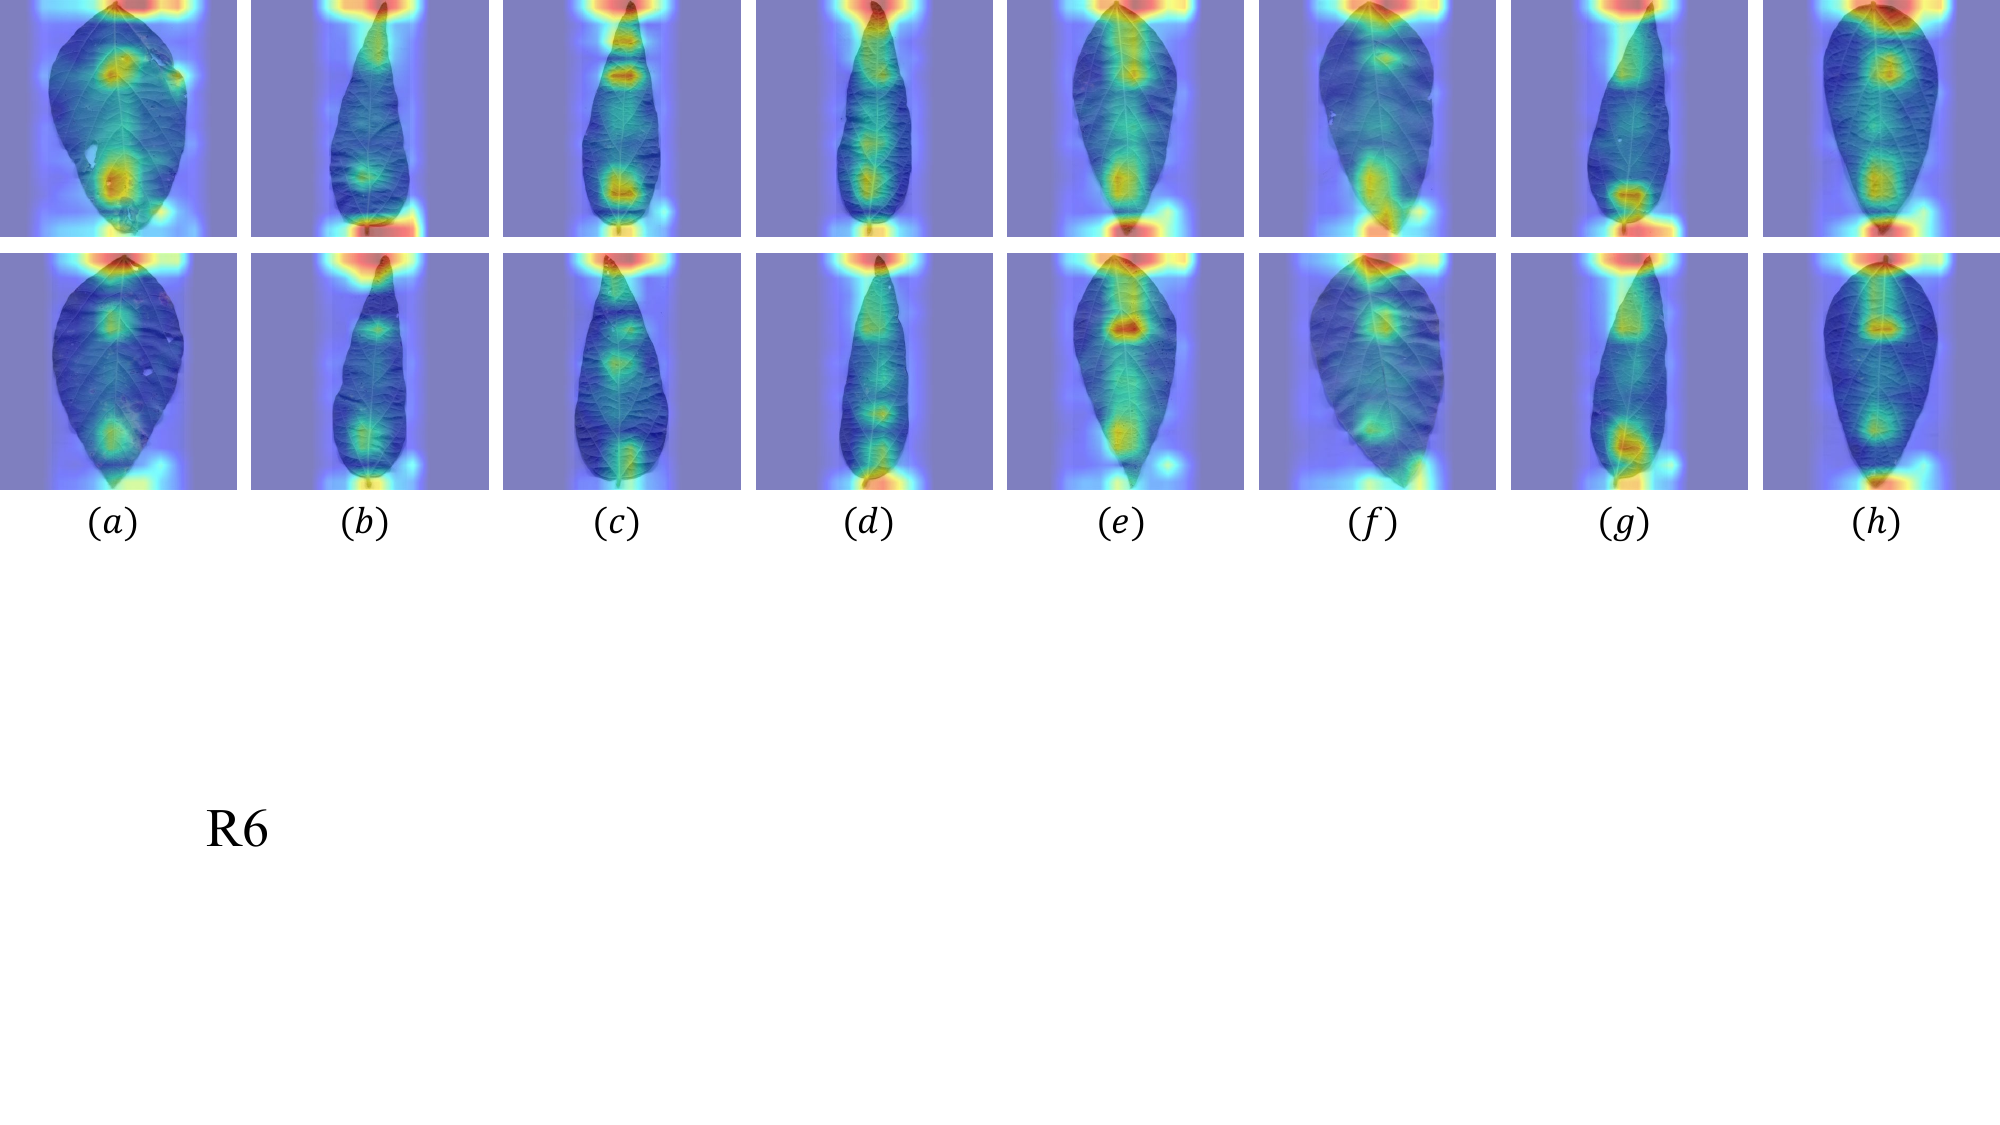}
   \caption{Visualization on 8 cultivars from SoyAgeing-R6.}
   \label{fig:cra-soyageing-r6}
  \end{subfigure}
  \caption{Visualization of top-15 groups of feature maps.}
  \label{fig:cra-visual-456}
\end{figure*}

%---------------------
% Experiments New
%---------------------
\begin{table*}[t]
\centering
  \begin{adjustbox}{width=1\linewidth}
%[width=\linewidth]1\linewidth
    \begin{tabular}{cccc|ccc|ccc|ccc}
      \toprule
      %Method & R1 & R3 & R4 & R5 & R6 \\
      \multirow{2}{*}{Method} & \multicolumn{3}{c|}{Cotton80} & \multicolumn{3}{c|}{SoyGene} & \multicolumn{3}{c|}{CUB-200-2011} & \multicolumn{3}{c}{Stanford Cars} \\ 
      & All & Old & New & All & Old & New & All & Old & New & All & Old & New \\%& All & Old & New & All & Old & New \\
      \midrule
      % RankStats+ & - & - & - & - & - & - & 66.10 & 80.70 & 51.80 & 56.3 & 81.8 & 31.7 \\
      UNO [7] & 28.25 & 17.50 & 39.00 & 28.68 & 44.21 & 13.15 & 43.79 & 68.30 & 19.27 
      & 51.81 & 81.17 & 22.45 \\
      IIC [16] & 32.19 & 30.00 & 34.38 & 30.16 & 51.60 & 8.91 & 41.57 & 65.05 & 18.09 & 52.87 & 84.35 & 21.38 \\
      %rKD & 41.67 & \textbf{46.67} & 36.67 & 19.05 & 33.71 & 4.52 & 53.69 & 86.61 & 21.94\\
      %rKD 32*448&  &  &  &  &  &  & 53.69 & 86.61 & 21.94\\
      \midrule
      %RAPL & 42.92 & 46.67 & 39.17 & 40.93 & 64.65 & 17.41 & 65.02 & 84.95 & 45.26\\
      RAPL & \textbf{42.92} & \textbf{46.67} & \textbf{39.17} & \textbf{40.93} & \textbf{64.65} & \textbf{17.41} & \textbf{56.42} & \textbf{81.11} & \textbf{32.29} & \textbf{64.41} & \textbf{85.61} & \textbf{43.40}\\%\textbf{65.45} & \textbf{93.19} & \textbf{38.70} \\
      %RAPL+ & - & - & - & - & - & - & 67.35 & 80.48 & 54.33\\
      %Ours W/SWA & 57.78 & 75.96 & 39.60 & 59.49 & 79.60 & 39.39 & 57.88 & 73.33 & 42.42 & 57.47 & 72.93 & 42.02 & 50.10 & 64.24 & 35.96 \\
      \bottomrule
       % &  \\
       % & 
    \end{tabular}
  \end{adjustbox}
\caption{Compared result of Cotton80, SoyGene and CUB.}
\label{tab:other dataset}
\end{table*}

\subsection{Feature Maps with CRA}
We provide the visualization of extracted feature maps in the test process after training by our RAPL in~\cref{fig:cra-visual-13}, where each column contains two visualizations of images from the same class. 
First, we extract feature maps $Z\in \mathbb{R}^{2048\times14\times14}$ with the model trained by our RAPL, and we generate the region representation $v^{r} \in \mathbb{R}^{196}$ with the maximum element after performing global max pooling on each group of feature maps $Z^i$, where each element $v^{r}_i$ is calculated by:
\begin{equation}
    v^{r}_i = \text{MAX}(\text{GMP}(\hat{Z}^i)).
    \label{eq:region_feature}
\end{equation}

Since we perform CRA on the final feature maps, \ie, $z\in \mathbb{R}^{14\times14}$, then each dimension of the feature map $z$ represents a 32 $\times$ 32 sized region of the input image.
However, as shown in~\cref{fig:cra-visual-13}, UFG images have white edges on both sides, which will lead to exactly the same features in these regions.
Thus we set the region representation of these blank regions to 0, and the improved representation is denoted as $\overline{v^r_i}$
Then, we visualize feature maps $\overline{Z}$ from the top 15 significant groups of feature maps excluding those blank regions, \ie
\begin{equation}
    %\begin{aligned}
        \overline{Z} = \{z^j \in \hat{Z}^i\}~~~~
        \text{s.t.}, i \in \{ i \mid \overline{v^r_i} \in \text{top-k}(\overline{v^r_i}) \},
    %\end{aligned}
\end{equation}
where $k=15$.
As shown in~\cref{fig:cra-visual-13,fig:cra-visual-456}, we can observe that the petiole and leaf tip are highlighted in most images. 
This is because these two parts contain rich texture information on leaf veins and shapes. 
Additionally, many highlighted areas are distributed around the main leaf veins, which 
indicates that our model automatically focuses on vein parts that are rich in texture information.
%is consistent with the motivation of manually designed methods based on leaf veins. 
Note that, with the constraints of our RAPL, the dominant features of instances that from the same class are distributed in similar regions of the images. 

Overall, the success of CRA can be summarized as follows: firstly, CRA aligns the feature channels in the same group into the assigned region. 
Then, RAPL compares different samples and proxies channel-wise, where the discriminative region features are preserved by the weights of aligned feature channels.
Since CRA learns different weights of channels in the group within the assigned region for different classes, thanks to the consistent region-channel alignment, these channels focus on the same region for both labeled and unlabeled classes.
Thus, the knowledge learned from labeled classes can be easily shared and transferred to discover novel classes of unlabeled samples.
\begin{table}[t]
\centering
  \begin{adjustbox}{width=1\linewidth}
%[width=\linewidth]1\linewidth
    \begin{tabular}{ccccccc}
      \toprule
      Method & R1 & R3 & R4 & R5 & R6 & AVG\\
      % \multirow{2}{*}{Method} & \multicolumn{3}{c}{R1} & \multicolumn{3}{c}{R3} & \multicolumn{3}{c}{R4} & \multicolumn{3}{c}{R5} & \multicolumn{3}{c}{R6} \\
      %   & All & Old & New & All & Old & New & All & Old & New & All & Old & New & All & Old & New \\
      \midrule
      % DCL [1] & 76.87 & 73.84 & 73.16 & 76.16 & 62.93 & 72.59 \\
      MaskCOV [30] & 79.80 & 74.65 & \textbf{79.60} & \textbf{78.28} & \textbf{66.97} & 75.86\\
      SPARE [32] & 78.28 & \textbf{79.90} & 78.69 & 77.27 & 64.44 & 75.72\\
      \midrule
      RAPL & \textbf{80.10} & 79.70 & 78.18 & 76.16 & 66.57 & \textbf{76.14}\\
      %Ours W/SWA & 57.78 & 75.96 & 39.60 & 59.49 & 79.60 & 39.39 & 57.88 & 73.33 & 42.42 & 57.47 & 72.93 & 42.02 & 50.10 & 64.24 & 35.96 \\
      \bottomrule
       % &  \\
       % & 
    \end{tabular}
  \end{adjustbox}
  %\vspace{-0.3cm}
\caption{Supervised classification for SoyAgeing series.}
\label{tab:supervise}
\end{table}

\begin{table}[t]
\centering
    \begin{adjustbox}{width=0.60\linewidth}
    \begin{tabular}{cc|ccc}
    \toprule
    \multicolumn{2}{c|}{Splits} & \multicolumn{3}{c}{SoyAgeing-R1} \\
    \cmidrule(lr){1-2}\cmidrule(lr){3-5}
    $C^l$ & $C^u$ & All & Old & New \\
    % & NCD & GCD & NCD & GCD & GCD \\
    \midrule
    33 & 165 & 40.61 & 61.21 & 36.48\\
    66 & 132 & 50.71 & 66.36 & 42.88\\
    99 & 99 & 58.99 & 79.19 & 38.79\\
    132 & 66 & 59.90 & 72.27& 35.15\\
    165 & 33 & 64.34 & 69.82 & 36.97\\
    \bottomrule
    \end{tabular}
    \end{adjustbox}
\caption{Illustrating the trend of performance on SoyAgeing-R1, when varying the numbers of labeled and unlabeled classes.}
\label{tab:split}
\end{table}

\subsection{More on Other Datasets}
The results in the~\cref{tab:other dataset} show that our RAPL consistently outperforms NCD methods by a large margin on other Ultra-FGVC (Cotton80 and SoyGene) and FGVC (CUB and S-Cars) datasets. We follow the same details to implement RAPL, UNO and IIC.
% except we set $\alpha=0.1$, $\beta=2$ when training RAPL for CUB and SCars. 
Note that, for a  fair comparison with RAPL on all the datasets, we
reproduce UNO and IIC with ResNet-50 rather than ViT-B/16.

\subsection{More on Supervised Learning}
As the Ultra-FGVC methods without the specific design for discovering new categories are not compatible with NCD, for a fair comparison, we adapt our RAPL into the conventional Ultra-FGVC image classification setting instead of UFG-NCD. In this case, all the samples are completely labeled, and we use them to train RAPL via the pre-train phase only. The results in the~\cref{tab:supervise} show that our RAPL is able to achieve competitive performance with state-of-the-art Ultra-FGVC methods as well.

%\noindent \textbf{Evaluation with Different Split Protocols.}
\subsection{More on Different Split Protocols}
To explore the effects of RAPL under strict annotation limitation, we train the network on varying splits of SoyAgeing-R1. The results in~\cref{tab:split} indicate that RAPL has strong robustness on unlabeled data despite the percentage of labeled classes.

% \begin{figure*}[t]
%   \centering
%    \includegraphics[width=1\linewidth]{pictures suppl/CRA_SoyAgeing-R1.pdf}
%    %\vspace{-0.55cm}
%    \caption{Visualization of feature maps $Z$ on SoyAgeing-R1 after train with CRA.
%    }
%    \label{fig:cra-soyageing-r1}
% \end{figure*}

% \begin{figure*}[b]
%   \centering
%    \includegraphics[width=1\linewidth]{pictures suppl/CRA_SoyAgeing-R3.pdf}
%    %\vspace{-0.55cm}
%    \caption{.
%    }
%    \label{fig:cra-soyageing-r3}
% \end{figure*}
